# Supplementary material for: Electrothermal Transistor Effect and Cyclic Electronic Currents in Multithermal Charge Transfer Networks
Source: arXiv:1908.00499 ancillary file (2019-08-01)
Supplement: Supplementary file 1 [file Supplement.pdf]

# Supplemental Material for "Electrothermal Transistor Effect and Cyclic Electronic Currents in Multithermal Charge Transfer Networks"

Galen T. Craven[1] and Abraham Nitzan[1,2]

[1]*Department of Chemistry, University of Pennsylvania, Philadelphia, PA 19104, USA*

[2]*School of Chemistry, Tel Aviv University, Tel Aviv 69978, Israel*

## I. DERIVATION OF THE MULTITHERMAL PROBABILITY DENSITY

We will now derive an expression for the probability density about the multidimensional transition state surface separating states in multithermal and multidimensional electron transfer reactions. The donor-acceptor networks we consider consist of $S$ total sites where each site $s$ can contain multiple modes, and each of these modes is in contact with a bath at the temperature of respective site $T_s$. The localized occupation by an electron on a particular site induces a unique electronic configuration in all the modes that "feel" the occupation of that site, thus the system also has $S$ total states. We will examine theoretically the reaction rate and coupled heat transfer during the transition from state $a$ to state $b$.

Adopting the Marcus formalism, the energy surface expression for a system in state $a$ is

$$E_a(x_1, \ldots, x_N) = E_a^{(0)} + \sum_s^S \sum_{j \in \mathcal{M}^{(s)}} \frac{1}{2} k_j \left( x_j - \lambda_j^{(a)} \right)^2, \tag{S1}$$

where $\mathcal{M}^{(s)}$ is the set of indices of all modes associated with the $s$th site, $k_j$ is the force constant of the $j$th mode, and $E_a^{(0)}$ is the electronic occupation energy of state $a$. The nuclear reconfiguration in the $j$th mode induced by a system in state $a$ is $\lambda_j^{(a)}$ and corresponds to an equilibrium shift in the parabolic energy surface of the respective mode. The total number of modes is denoted by $N$ and the total number of modes associated with site $s$ is $N_s$. The set of indices of all of all modes is $\mathcal{M} \subseteq \mathbb{Z}^+$ and $\mathcal{M} = \mathcal{M}^{(1)} \cup \mathcal{M}^{(2)} \cup \ldots \cup \mathcal{M}^{(S)}$. Note that $\mathcal{M}^{(i)} \cap \mathcal{M}^{(j)} = \varnothing$ for all $i \neq j$ and thus the sets corresponding to different sites are disjoint. For the process $a \to b$ (which for notational convenience we will sometimes denote as $a, b$), the difference between the equilibrium position of the $j$th mode in state $a$ and in state $b$ is

$$\Delta\lambda_j = \lambda_j^{(a)} - \lambda_j^{(b)}. \tag{S2}$$

The reference state of each oscillator is

$$E_{\text{ref}}(x_j) = \frac{1}{2} k_j x_j^2, \tag{S3}$$

The reference state of the system is

$$E_{\mathrm{ref}}^{(\mathrm{sys})}(x_1,\ldots,x_N) = \sum_j^N \frac{1}{2} k_j x_j^2, \tag{S4}$$

and corresponds to the absence of an electron. The electron occupation of site $a$ is defined as state $a$ and corresponds to the electron being felt by all modes not in the reference state in $E_a$. The condition for adiabatic electron transfer is $E_a = E_b$, i.e., the energy of the system is conserved during the state transition. For the *forward* $a \to b$ process, the free energy of the reaction is $E_{ba} = E_b^{(0)} - E_a^{(0)}$, and for the *backward* $b \to a$ process the free energy is $E_{ab} = E_a^{(0)} - E_b^{(0)}$. The reorganization energy of the $j$th mode and the total reorganization energy are

$$E_{\mathrm{R}j}^{(a,b)} = \frac{1}{2} k_j \Delta\lambda_j^2 \quad \text{and} \quad E_{\mathrm{R}}^{(a,b)} = \sum_j^N E_{\mathrm{R}j} \tag{S5}$$

respectively.

The transition state structure for the reaction $a \to b$ (and also $b \to a$) is formed by the set of points are where the energy surfaces $E_a$ and $E_b$ are equienergetic. Due to the paraboloid geometry of the respective energy surfaces given by Eq. (S1), this transition state is a hypersurface. The equation for the transition surface (TS) can be written as

$$g_{\mathrm{c}}(x_1,\ldots,x_N) = E_b(x_1,\ldots,x_N) - E_a(x_1,\ldots,x_N) = \sum_j^N k_j \Delta\lambda_j x_j + E' = 0, \tag{S6}$$

where

$$E' = E_{ba} + \frac{1}{2} \sum_j^N k_j \left(\lambda_j^{(b)} + \lambda_j^{(a)}\right) \left(\lambda_j^{(b)} - \lambda_j^{(a)}\right). \tag{S7}$$

The gradient magnitude of this hyperplane is

$$|\nabla g_{\mathrm{c}}| = \sqrt{\sum_j^N (k_j \Delta\lambda_j)^2} = \sqrt{2 \sum_j^N k_j E_{\mathrm{R}j}^{(a,b)}}. \tag{S8}$$

The probability density term in the rate expression given by $k_{a,b} = \frac{1}{2} \langle \mathcal{T}_{a,b}\, \dot{x}_\perp \rangle P_{a,b}$ can be written using the Dirac $\delta$-function to constrain the integration over the TS as

$$P_{a,b} = \frac{\displaystyle\int_{\mathbb{R}^N} |\nabla g_{\mathrm{c}}|\, \delta\Big(E_b(x_1,\ldots,x_N) - E_a(x_1,\ldots,x_N)\Big) \prod_s^S \prod_{j\in\mathcal{M}^{(s)}} \exp\left[-\beta_s \frac{1}{2} k_j \left(x_j - \lambda_j^{(a)}\right)^2\right] dx_j}{\displaystyle\int_{\mathbb{R}^N} \prod_s^S \prod_{j\in\mathcal{M}^{(s)}} \exp\left[-\beta_s \frac{1}{2} k_j \left(x_j - \lambda_j^{(a)}\right)^2\right] dx_j}, \tag{S9}$$

where $\beta_s = 1/k_\mathrm{B}T_s$ is the inverse thermal energy of the bath that is in contact with the $s$th site and $k_\mathrm{B}$ is Boltzmann's constant. The factor $|\nabla g_\mathrm{c}|$ in Eq. (S9) arises from the coarea formula and removes ambiguity in the $\delta$-function constraint [**?** **?** ]. The $\delta$-function can be expressed in integral form as

$$\delta\Big(E_b(x_1,\ldots,x_N)-E_a(x_1,\ldots,x_N)\Big) = \frac{1}{2\pi}\int_{\mathbb{R}} \exp\left[i\Big(E_b(x_1,\ldots,x_N)-E_a(x_1,\ldots,x_N)\Big)\tau\right] d\tau \quad \text{(S10)}$$

and thus the the probability density expression can be written as a product of integrals over $S$ sites,

$$P_{a,b} = \frac{\displaystyle\int_{\mathbb{R}} |\nabla g_\mathrm{c}| \exp\left[iE'\tau\right] \prod_s^S \int_{\mathbb{R}^{N_s}} \prod_{j\in\mathcal{M}^{(s)}} \exp\left[-\beta_s \frac{1}{2}k_j\left(x_j-\lambda_j^{(a)}\right)^2 + ik_j\Delta\lambda_j x_j\tau\right] dx_j\, d\tau}{\displaystyle 2\pi \prod_s^S \int_{\mathbb{R}^{N_s}} \prod_{j\in\mathcal{M}^{(s)}} \exp\left[-\beta_s \frac{1}{2}k_j\left(x_j-\lambda_j^{(a)}\right)^2\right] dx_j}. \quad \text{(S11)}$$

Repeated application of Fubini's theorem allows the multidimensional integral to be written as

$$P_{a,b} = \frac{\displaystyle\int_{\mathbb{R}} |\nabla g_\mathrm{c}| \exp\left[iE'\tau\right] \prod_s^S \left(\prod_{j\in\mathcal{M}^{(s)}} \int_{\mathbb{R}} \exp\left[-\beta_s \frac{1}{2}k_j\left(x_j-\lambda_j^{(a)}\right)^2 + ik_j\Delta\lambda_j x_j\tau\right] dx_j\right) d\tau}{\displaystyle 2\pi \prod_s^S \left(\prod_{j\in\mathcal{M}^{(s)}} \int_{\mathbb{R}} \exp\left[-\beta_s \frac{1}{2}k_j\left(x_j-\lambda_j^{(a)}\right)^2\right] dx_j\right)}, \quad \text{(S12)}$$

which can also be expressed as a single product of integrals over all $N$ modes,

$$P_{a,b} = \frac{\displaystyle\int_{\mathbb{R}} |\nabla g_\mathrm{c}| \exp\left[iE'\tau\right] \left(\prod_j^N \int_{\mathbb{R}} \exp\left[-\beta_j \frac{1}{2}k_j\left(x_j-\lambda_j^{(a)}\right)^2 + ik_j\Delta\lambda_j x_j\tau\right] dx_j\right) d\tau}{\displaystyle 2\pi \left(\prod_j^N \int_{\mathbb{R}} \exp\left[-\beta_j \tfrac{1}{2}k_j\left(x_j-\lambda_j^{(a)}\right)^2\right] dx_j\right)}. \quad \text{(S13)}$$

Note that $\beta_j = \beta_s$ for $j \in \mathcal{M}^{(s)}$ and in the limit $N \to \infty \Rightarrow \mathcal{M} = \mathbb{Z}^+$.

A succinct form of the the probability density expression can be written by noting that the argument of the exponential functions in Eq. (S13) can be written as

$$\mathcal{F}_j(x_j,\tau) = -\beta_j \tfrac{1}{2}k_j\left(x_j-\lambda_j^{(a)}\right)^2 + ik_j\Delta\lambda_j x_j\tau. \quad \text{(S14)}$$

The real part $\Re(\mathcal{F})$ of this function arises from the configuration integrals over each mode and the imaginary part $\Im(\mathcal{F})$ from the integral form of the $\delta$-function constraint. Note that

$\partial_\tau \Re\big[\mathcal{F}_j(x_j,\tau)\big] = 0$. The probability density expression can now be written as

$$P_{a,b} = \frac{\displaystyle\int_{\mathbb{R}} |\nabla g_{\rm c}| \exp\Big[iE'\tau\Big] \left(\prod_j^N \int_{\mathbb{R}} \exp\Big[\mathcal{F}_j(x_j,\tau)\Big]\, dx_j\right) d\tau}{\displaystyle 2\pi \prod_j^N \int_{\mathbb{R}} \exp\Big[\Re\big[\mathcal{F}_j(x_j,\tau)\big]\Big]\, dx_j}. \tag{S15}$$

After evaluating the configuration-space integrals corresponding to $x_j \in \mathcal{M}$, we arrive at

$$\begin{aligned} P_{a,b} &= \frac{|\nabla g_{\rm c}|}{2\pi} \int_{\mathbb{R}} \exp\Big[iE'\tau\Big] \prod_j^N \exp\left[-\frac{k_j \Delta\lambda_j^2}{2\beta_j}\tau^2 + i k_j \lambda_j^{(a)} \Delta\lambda_j \tau\right] d\tau \\ &= \frac{|\nabla g_{\rm c}|}{2\pi} \int_{\mathbb{R}} \prod_j^N \exp\left[-\frac{k_j \Delta\lambda_j^2}{2\beta_j}\tau^2 + i\left(k_j \lambda_j^{(a)} \Delta\lambda_j + E'\right)\tau\right] d\tau, \end{aligned} \tag{S16}$$

which can be written in terms of the parameters

$$\alpha = \sum_j^N \frac{k_j \Delta\lambda_j^2}{2\beta_j} \quad \text{and} \quad \gamma = E' + \sum_j^N k_j \lambda_j^{(a)} \Delta\lambda_j \tag{S17}$$

as

$$\begin{aligned} P_{a,b} &= \frac{|\nabla g_{\rm c}|}{2\pi} \int_{\mathbb{R}} \exp\Big[-\alpha\tau^2 + i\gamma\tau\Big]\, d\tau \\ &= \frac{|\nabla g_{\rm c}|}{2} \sqrt{\frac{1}{\pi\alpha}} \exp\left[-\frac{\gamma^2}{4\alpha}\right]. \end{aligned} \tag{S18}$$

Evaluation then leads to the expression

$$\begin{aligned} P_{a,b} = |\nabla g_{\rm c}| &\sqrt{\prod_l^N \beta_l \Bigg/ \left(2\pi \sum_j^N k_j \Delta\lambda_j^2 \prod_{l\neq j}^N \beta_l\right)} \\ &\times \exp\left[-\left(\prod_l^N \beta_l\right)\left(E' + \sum_q^N k_q \lambda_q^{(a)} \Delta\lambda_q\right)^2 \Bigg/ 2\sum_j^N \left(\prod_{l\neq j}^N \beta_l\right) k_j \Delta\lambda_j^2\right]. \end{aligned} \tag{S19}$$

After some algebra and substitution for $E'$ we obtain

$$\begin{aligned} P_{a,b} = &\sqrt{\sum_j^N k_j E_{{\rm R}j}^{(a,b)} \prod_l^N \beta_l \Bigg/ 2\pi \sum_j^N E_{{\rm R}j}^{(a,b)} \prod_{l\neq j}^N \beta_l} \\ &\times \exp\left[-\left(E_{ba} + E_{\rm R}^{(a,b)}\right)^2 \prod_l^N \beta_l \Bigg/ 4\sum_j^N E_{{\rm R}j}^{(a,b)} \prod_{l\neq j}^N \beta_l\right]. \end{aligned} \tag{S20}$$

Expressing each $\beta_j$ factor in terms of the corresponding temperature $T_j$, and writing the expression

as a sum over all sites yields

$$P_{a,b} = \sqrt{\sum_j^N k_j E_{\mathrm{R}j}^{(a,b)} \Bigg/ 2\pi k_\mathrm{B} \sum_s^S T_s \sum_{j\in\mathcal{M}^{(s)}} E_{\mathrm{R}j}^{(a,b)}} \\ \times \exp\left[ -\left(E_{ba} + E_\mathrm{R}^{(a,b)}\right)^2 \Bigg/ 4k_\mathrm{B} \sum_s^S T_s \sum_{j\in\mathcal{M}^{(s)}} E_{\mathrm{R}j}^{(a,b)} \right], \tag{S21}$$

which is the multithermal probability density about the TS for the state transition $a \to b$.

## II. MULTITHERMAL NORMAL VELOCITY

Associated with each of the $N$ modes is a single degree-of-freedom $x_j : j \in \mathcal{M}$, and thus the state of the system can be specified through the vector

$$\mathbf{x} = \{x_1, x_2, \ldots, x_N\}. \tag{S22}$$

The state vector $\mathbf{x}$ has a corresponding velocity vector

$$\dot{\mathbf{x}} = \{\dot{x}_1, \dot{x}_2, \ldots, \dot{x}_N\}, \tag{S23}$$

where $\dot{x}_j$ is the velocity of the respective mode. Each mode has an associated mass $m_j$. We want to calculate the multithermal expectation value of the velocity normal to the TSHP, which is a subspace that contains all points where the surfaces $E_a$ and $E_b$ are equienergetic. A unit normal vector to the TS is

$$\hat{\mathbf{u}}_\perp = \{n_1, n_2, \ldots, n_N\} = \left\{ \frac{k_1 \Delta\lambda_1}{|\nabla g_\mathrm{c}|}, \frac{k_2 \Delta\lambda_2}{|\nabla g_\mathrm{c}|}, \ldots, \frac{k_N \Delta\lambda_N}{|\nabla g_\mathrm{c}|} \right\}. \tag{S24}$$

The velocity vector $\dot{\mathbf{x}}$ has a scalar component in the direction of the normal,

$$\dot{x}_\perp(\dot{x}_1, \dot{x}_2, \ldots, \dot{x}_N) = \dot{\mathbf{x}} \cdot \hat{\mathbf{u}}_\perp = \dot{x}_1 n_1 + \dot{x}_2 n_2 + \ldots + \dot{x}_N n_N. \tag{S25}$$

We want to calculate the expectation value of this normal component

$$\langle \dot{x}_\perp \rangle = \frac{\displaystyle\int_\mathcal{C} \dot{x}_\perp(\dot{x}_1, \ldots, \dot{x}_N) \prod_j^N \exp\left[-\beta_j \left(\frac{1}{2} m_j \dot{x}_j^2\right)\right] d\dot{x}_j}{\displaystyle\int_\mathcal{C} \prod_j^N \exp\left[-\beta_j \left(\frac{1}{2} m_j \dot{x}_j^2\right)\right] d\dot{x}_j}, \tag{S26}$$

over the constrained subspace $\mathcal{C}$ where $\dot{x}_\perp \geq 0$, i.e., we want to include only nonnegative values of the scalar velocity component in the direction of the normal in the expectation value calculation.

This constraint can be enforced using the Heaviside function,

$$\langle \dot{x}_\perp \rangle = \frac{\displaystyle\int_{\mathbb{R}^N} \dot{x}_\perp(\dot{x}_1,\ldots,\dot{x}_N)\ \Theta\Big(\dot{x}_\perp(\dot{x}_1,\ldots,\dot{x}_N)\Big) \prod_j^N \exp\left[-\beta_j \left(\frac{1}{2}m_j\dot{x}_j^2\right)\right] d\dot{x}_j}{\displaystyle\int_{\mathbb{R}^N} \Theta\Big(\dot{x}_\perp(\dot{x}_1,\ldots,\dot{x}_N)\Big) \prod_j^N \exp\left[-\beta_j \left(\frac{1}{2}m_j\dot{x}_j^2\right)\right] d\dot{x}_j}. \tag{S27}$$

Expressing the Heaviside function in integral form and expanding the normal velocity in terms of the respective components $\dot{x}_1, \dot{x}_2, \ldots, \dot{x}_N$ gives,

$$\langle \dot{x}_\perp \rangle = \frac{\displaystyle\lim_{\epsilon\to 0}\int_{\mathbb{R}}\int_{\mathbb{R}^N} \frac{1}{\tau - i\epsilon}\Big(\dot{x}_1 n_1 + \ldots + \dot{x}_N n_N\Big) \prod_j^N \exp\left[-\beta_j \left(\frac{1}{2}m_j\dot{x}_j^2\right) + i n_j \dot{x}_j \tau\right] d\dot{x}_j d\tau}{\displaystyle\lim_{\epsilon\to 0}\int_{\mathbb{R}}\int_{\mathbb{R}^N} \frac{1}{\tau - i\epsilon} \prod_j^N \exp\left[-\beta_j \left(\frac{1}{2}m_j\dot{x}_j^2\right) + i n_j \dot{x}_j \tau\right] d\dot{x}_j d\tau}. \tag{S28}$$

By recursive application of Fubini's theorem, the expectation integral can be written as

$$\begin{aligned}\langle \dot{x}_\perp \rangle = \lim_{\epsilon\to 0}\int_{\mathbb{R}} \frac{1}{\tau - i\epsilon} \sum_j^N \int_{\mathbb{R}} \dot{x}_j n_j \exp\left[-\beta_j \left(\frac{1}{2}m_j\dot{x}_j^2\right) + i n_j \dot{x}_j \tau\right] \\ \times \left(\prod_{l\neq j}^N \int_{\mathbb{R}} \exp\left[-\beta_l \left(\frac{1}{2}m_l\dot{x}_l^2\right) + i n_l \dot{x}_l \tau\right] d\dot{x}_l\right) d\dot{x}_j d\tau \\ \Bigg/ \lim_{\epsilon\to 0}\int_{\mathbb{R}} \frac{1}{\tau - i\epsilon} \left(\prod_j^N \int_{\mathbb{R}} \exp\left[-\beta_j \left(\frac{1}{2}m_j\dot{x}_j^2\right) + i n_j \dot{x}_j \tau\right] d\dot{x}_j\right) d\tau.\end{aligned} \tag{S29}$$

Linearity of integration allows the expectation value calculation to to be organized as

$$\begin{aligned}\langle \dot{x}_\perp \rangle = \sum_j^N \lim_{\epsilon\to 0}\int_{\mathbb{R}} \frac{1}{\tau - i\epsilon} \int_{\mathbb{R}} \dot{x}_j n_j \exp\left[-\beta_j \left(\frac{1}{2}m_j\dot{x}_j^2\right) + i n_j \dot{x}_j \tau\right] \\ \times \left(\prod_{l\neq j}^N \int_{\mathbb{R}} \exp\left[-\beta_l \left(\frac{1}{2}m_l\dot{x}_l^2\right) + i n_l \dot{x}_l \tau\right] d\dot{x}_l\right) d\dot{x}_j d\tau \\ \Bigg/ \lim_{\epsilon\to 0}\int_{\mathbb{R}} \frac{1}{\tau - i\epsilon} \left(\prod_l^N \int_{\mathbb{R}} \exp\left[-\beta_l \left(\frac{1}{2}m_l\dot{x}_l^2\right) + i n_l \dot{x}_l \tau\right] d\dot{x}_l\right) d\tau.\end{aligned} \tag{S30}$$

Upon evaluation of the integrals, and by inductive reasoning, we arrive at

$$\langle \dot{x}_\perp \rangle = \sum_j^N \frac{n_j^2}{m_j\beta_j} \sqrt{2\prod_l^N \beta_l m_l \Bigg/ \pi \sum_k^N n_k^2 \prod_{l\neq k}^N \beta_l m_l}, \tag{S31}$$

which reduces to the form

$$\langle \dot{x}_\perp \rangle = \sqrt{2\sum_j^N n_j^2 \prod_{l\neq j}^N \beta_l m_l \Bigg/ \pi \prod_l^N \beta_l m_l}. \tag{S32}$$

Writing this in terms of the bath temperatures gives

$$\langle \dot{x}_\perp \rangle = \sqrt{2k_\mathrm{B} \sum_j^N n_j^2 T_j \Big/ \pi m_j}, \tag{S33}$$

which reduces to

$$\langle \dot{x}_\perp \rangle = \sqrt{2k_\mathrm{B} \sum_s^S T_s \sum_{j\in\mathcal{M}^{(s)}} n_j^2 \Big/ \pi m_j}. \tag{S34}$$

Expressing the normal components in terms of the corresponding force constants and reorganization energies yields

$$\langle \dot{x}_\perp \rangle = \sqrt{4k_\mathrm{B} \sum_s^S T_s \sum_{j\in\mathcal{M}^{(s)}} k_j E_{\mathrm{R}j}^{(a,b)} \Big/ \left|\nabla g_\mathrm{c}\right|^2 \pi m_j}, \tag{S35}$$

which is the expected value of the the velocity component normal to the TS.

## III. TUNNELING PROBABILITY

In the adiabatic limit, the tunneling probability $\mathcal{T}_{a,b} = 1$ and thus the frequency term in the rate expression is proportional to $\langle \dot{x}_\perp \rangle$, which is derived in Section II. In the nonadiabatic limit, the tunneling probability between states $a$ and $b$ can be approximated using the Landau-Zener (LZ) formula:

$$\mathcal{T}_{a,b}^{\mathrm{LZ}} = 1 - \exp\left[-\frac{2\pi H_{a,b}^2}{\hbar|\Delta F|\dot{x}_\perp}\right], \tag{S36}$$

where $H_{a,b}$ is the coupling constant between adiabatic energy surfaces and $|\Delta F|$ is the difference in the forces normal to the TS on each surface [? ? ? ]. The LZ formula is only valid in one dimension but can be used in multidimensional problems by evaluating in the direction normal the TSHP [? ]. For paraboloid energy surfaces,

$$|\Delta F| = |\nabla(E_b - E_a)| = \left|\nabla g_\mathrm{c}\right|. \tag{S37}$$

A first-order approximation to $\mathcal{T}_{a,b}^{\mathrm{LZ}}$ yields

$$\mathcal{T}_{a,b} = \frac{2\pi\Delta H_{a,b}^2}{\hbar|\Delta F|\dot{x}_\perp}. \tag{S38}$$

In this limit $\mathcal{T}_{a,b} \propto 1/\dot{x}_\perp$, and the expectation value $\langle \mathcal{T}_{a,b}\, \dot{x}_\perp \rangle$ does not depend on the normal velocity.

## IV. MULTITHERMAL HEAT TRANSFER DERIVATION

The heat transferred during the $a \to b$ state transition is

$$\mathcal{Q}^{(a,b)}\Big(\boldsymbol{x}^{\mathrm{TS}}\Big) = -\mathcal{Q}^{(a)}_{\mathrm{obt}}\Big(\boldsymbol{x}^{\mathrm{TS}}\Big) + \mathcal{Q}^{(b)}_{\mathrm{rel}}\Big(\boldsymbol{x}^{\mathrm{TS}}\Big). \tag{S39}$$

where $\boldsymbol{x}^{\mathrm{TS}} = \{x_1, \ldots, x_N\} : E_b(x_1, \ldots, x_N) - E_a(x_1, \ldots, x_N) = 0$ is a specific point on the TS, $\mathcal{Q}^{(a)}_{\mathrm{obt}}$ is the heat obtained from the bath during the ascent to $\boldsymbol{x}$ on the $E_a$ surface, and $\mathcal{Q}^{(b)}_{\mathrm{rel}}$ is the heat released on the $E_b$ energy surface during the descent to equilibrium. For the $a \to b$ transition the heat transferred to the $j$th bath can be written as

$$\mathcal{Q}^{(a,b)}_j\Big(x_j \in \boldsymbol{x}^{\mathrm{TS}}\Big) = -\frac{1}{2}k_j\left[x_j - \lambda^{(a)}_j\right]^2 + \frac{1}{2}k_j\left[x_j - \lambda^{(b)}_j\right]^2. \tag{S40}$$

The expectation value for the heat transferred in the $j$th bath is

$$\Big\langle \mathcal{Q}^{(a,b)}_j \Big\rangle = \int_{\mathbb{R}^N} \mathcal{Q}^{(a,b)}_j \, P^{\ddagger}_a(x_1, \ldots, x_N)\, dx_1 \ldots dx_N, \tag{S41}$$

where

$$P^{\ddagger}_{a,b}(x_1, \ldots, x_N) = \frac{\delta\Big(E_b(x_1, \ldots, x_N) - E_a(x_1, \ldots, x_N)\Big)\displaystyle\prod_j^N \exp\left[-\beta_j \frac{1}{2}k_j\left(x_j - \lambda^{(a)}_j\right)^2\right]}{\displaystyle\int_{\mathbb{R}^N} \delta\Big(E_b(x_1, \ldots, x_N) - E_a(x_1, \ldots, x_N)\Big)\prod_j^N \exp\left[-\beta_j \frac{1}{2}k_j\left(x_j - \lambda^{(a)}_j\right)^2\right] dx_j}, \tag{S42}$$

is the probability density *restricted* to the TS. Using the integral form of the $\delta$-function and the $\mathcal{F}$ function defined in Section I, this multithermal probability density can be written as

$$P^{\ddagger}_{a,b}(x_1, \ldots, x_N) = \frac{\displaystyle\int_{\mathbb{R}} \exp\Big[iE'\tau\Big] \prod_j^N \exp\Big[\mathcal{F}_j(x_j, \tau)\Big]\, d\tau}{\displaystyle\int_{\mathbb{R}} \exp\Big[iE'\tau\Big] \left(\prod_j^N \int_{\mathbb{R}} \exp\Big[\mathcal{F}_j(x_j, \tau)\Big]\, dx_j\right) d\tau}. \tag{S43}$$

Combining Eqs. (**??**), (**??**), and (**??**) gives

$$\Big\langle \mathcal{Q}^{(a,b)}_l \Big\rangle = \frac{\displaystyle\int_{\mathbb{R}^2} \exp\Big[iE'\tau\Big] \mathcal{Q}^{(a,b)}_l \exp\Big[\mathcal{F}_l(x_l, \tau)\Big] \left(\prod_{j\neq l}^{N-1} \int_{\mathbb{R}} \exp\Big[\mathcal{F}_j(x_j, \tau)\Big]\, dx_j\right) dx_l\, d\tau}{\displaystyle\int_{\mathbb{R}} \exp\Big[iE'\tau\Big] \left(\prod_j^N \int_{\mathbb{R}} \exp\Big[\mathcal{F}_j(x_j, \tau)\Big]\, dx_j\right) d\tau}, \tag{S44}$$

and after evaluating the integrals we obtain

$$\left\langle \mathcal{Q}_j^{(a,b)} \right\rangle = \frac{-E_{\mathrm{R}j}^{(a,b)} \left[ E_{ba} \prod_{l\neq j}^{N} \beta_l + \sum_{k\neq j}^{N} E_{\mathrm{R}k}^{(a,b)} \left( \beta_k - \beta_j \right) \prod_{l\notin\{j,k\}}^{N} \beta_l \right]}{\sum_{k}^{N} E_{\mathrm{R}k}^{(a,b)} \prod_{l\neq k}^{N} \beta_l}, \tag{S45}$$

which is the expected heat transferred to bath associated with the $j$th mode during the state transition $a \to b$. Written in terms of the temperatures the expression can be reduced to

$$\left\langle \mathcal{Q}_j^{(a,b)} \right\rangle = \frac{E_{\mathrm{R}j}^{(a,b)} \left[ E_{ab} T_j + \sum_{k}^{N} E_{\mathrm{R}k}^{(a,b)} \left( T_k - T_j \right) \right]}{\sum_{k}^{N} E_{\mathrm{R}k}^{(a,b)} T_k}. \tag{S46}$$

For a specific site $s$, the heat transferred into the corresponding bath is the sum of all modes associated with that site:

$$\left\langle \mathcal{Q}_s^{(a,b)} \right\rangle = \sum_{j\in\mathcal{M}^{(s)}} \left\langle \mathcal{Q}_j^{(a,b)} \right\rangle, \tag{S47}$$

which can be written by applying Eq. (**??**) as

$$\left\langle \mathcal{Q}_s^{(a,b)} \right\rangle = \frac{\sum_{j\in\mathcal{M}^{(s)}} E_{\mathrm{R}j}^{(a,b)} \left[ E_{ab}\, T_s + \sum_{q\neq s}^{S} \sum_{k\in\mathcal{M}^{(q)}} E_{\mathrm{R}k}^{(a,b)} \left( T_q - T_s \right) \right]}{\sum_{q}^{S} T_q \sum_{k\in\mathcal{M}^{(q)}} E_{\mathrm{R}k}^{(a,b)}}. \tag{S48}$$

In the specific case of a system with the same reorganization energy $E_{\mathrm{R}}^{*}$ in each mode, the heat transferred into the bath associated with the $s$th site is

$$\left\langle \mathcal{Q}_s^{(a,b)} \right\rangle = \frac{N_s \left[ E_{ab}\, T_s + E_{\mathrm{R}}^{*} \sum_{q\neq s}^{S} N_q \left( T_q - T_s \right) \right]}{\sum_{q}^{S} N_q T_q}. \tag{S49}$$

where $N_s$ and $N_q$ are the number of modes in equilibrium with the baths associated with site $s$ and site $q$, respectively. As an example, consider the specific case of two sites (1 and 2) with $N_1$ and $N_2$ modes associated with the respective site. The heat transferred into bath 1 during the $a \to b$ transition is

$$\left\langle \mathcal{Q}_1^{(a,b)} \right\rangle = \frac{E_{ab} N_1 T_1 + E_{\mathrm{R}}^{*} N_1 N_2 \left( T_2 - T_1 \right)}{N_1 T_1 + N_2 T_2}, \tag{S50}$$

and correspondingly for bath 2:

$$\left\langle \mathcal{Q}_2^{(a,b)} \right\rangle = \frac{E_{ab} N_2 T_2 + E_{\mathrm{R}}^* N_1 N_2 \left(T_1 - T_2\right)}{N_1 T_1 + N_2 T_2}. \tag{S51}$$

The sum of these terms is

$$\left\langle \mathcal{Q}_1^{(a,b)} \right\rangle + \left\langle \mathcal{Q}_2^{(a,b)} \right\rangle = E_{ab}, \tag{S52}$$

which illustrates the conservation of energy as $E_{ba} = -E_{ab}$ is the free energy of the reaction.

## V. ANALYSIS OF EXAMPLE COMPLEX NETWORKS

The developed theory can be applied to describe thermal and electronic transport in more complex networks of donors and acceptors than the $\mathcal{R}_3$ network analyzed in the main text. As

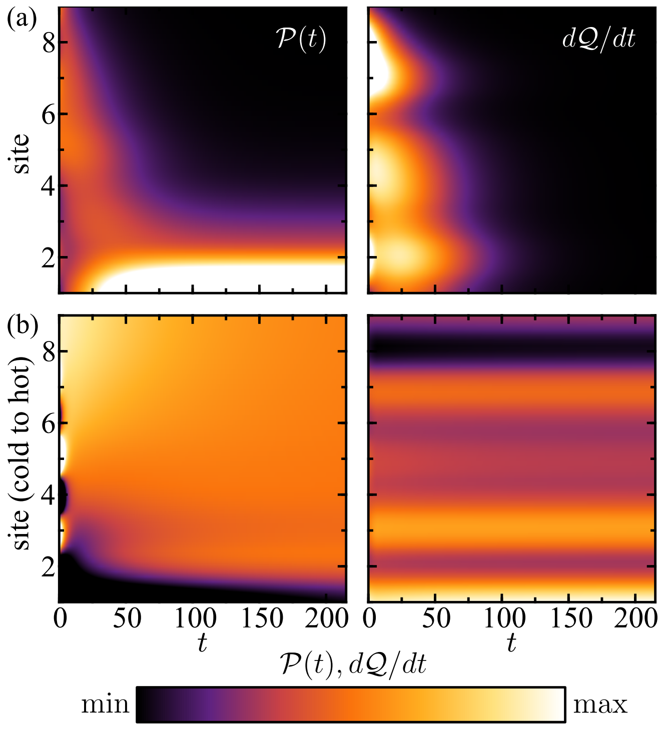


FIG. S1. Density plots of the site population $\mathcal{P}$ (left) and corresponding heat current $d\mathcal{Q}/dt$ (right) at steady-state in each site as function of time for a nine-site $\mathcal{L}$ network with: (a) no temperature gradient ($T_a = 1 \,\forall\, a$) and a monotonically-ramped electronic energy landscape $E_a^{(0)} \in [-5, 5]$ and (b) a linear temperature gradient $T_a \in [1/10, 2]$ and a flat energy landscape $E_a^{(0)} = 0 \,\forall\, a$. All modes have the same mass and frequency. In both (a) and (b) specific realizations of $\lambda$ values (generated by randomly sampling from a uniform distribution over the interval $[-1, 1]$) are shown. All quantities are shown in reduced units and calculated in the adiabatic limit.

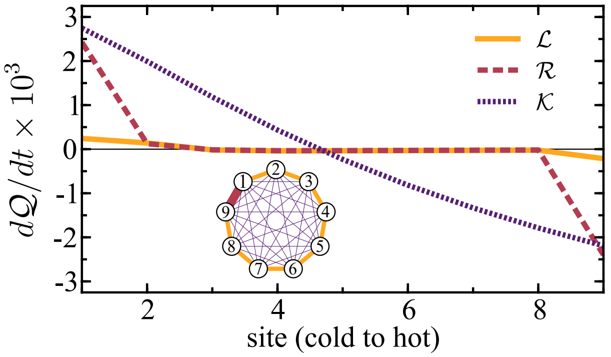


FIG. S2. Heat current $d\mathcal{Q}/dt$ at steady-state for each site of a nine-site network calculated for various topologies with each network having a flat energy landscape $E_a^{(0)} = 0\,\forall\, a$ and linear temperature gradient $T_s \in [1/10, 2]$. All reorganization energies are $E_{\mathrm{R}j} = 1$ for each mode involved in a particular a transition and zero otherwise. The ordering of the sites is shown in the inset with edge colors corresponding to the respective network topology. Note that $\mathcal{L}$ is a subgraph of $\mathcal{R}$, and both are subgraphs of $\mathcal{K}$. The currents are scaled by the total number of connections in each network. All calculations are in the adiabatic limit.

illustrated in Fig. **??**(a) for a nine-site $\mathcal{L}$ network, in unithermal systems the occupation probabilities are dictated only by the energy landscape, and the site with the lowest electronic energy will have the highest probability of occupation, in accordance with expected statistical mechanics. In contrast, if a system is characterized by multiple local temperatures, the occupation probabilities are dictated by relations between the thermal gradient and the electronic landscape. The heat currents in Fig. **??**(a) illustrate that in unithermal systems at steady-state the heat currents vanish ($\dot{\mathcal{Q}}_a = 0\,\forall\, a$). In contrast, for multithermal systems, striated thermal patterns emerge as shown in Fig. **??**(b).

The induced multithermal heat and electronic currents depend on the topology of the underlying network, with distinct variations arising from specific connectivities. As shown in Fig. **??**, in a linear $\mathcal{L}$ network, the heat flow is unidirectional across all sites with the coldest bath acting as a heat sink for the system. For $\mathcal{R}$ topology, a local current is induced by connecting the coldest and hottest sites. The heat current through the ring system is small compared to the large local current from the coldest site to the neighboring hottest site. The $\mathcal{K}$ network is topologically invariant and thus the heat current form is dictated by the temperature gradient and its relation to the reorganization energy in each mode.

As noted in the main text, in cyclic multithermal systems the unidirectional flux through a specific connection $a \to b$ is not necessarily equal to the flux through the reverse connection $b \to a$, which is contrast to the unithermal case where the net flux through a connection always vanishes.

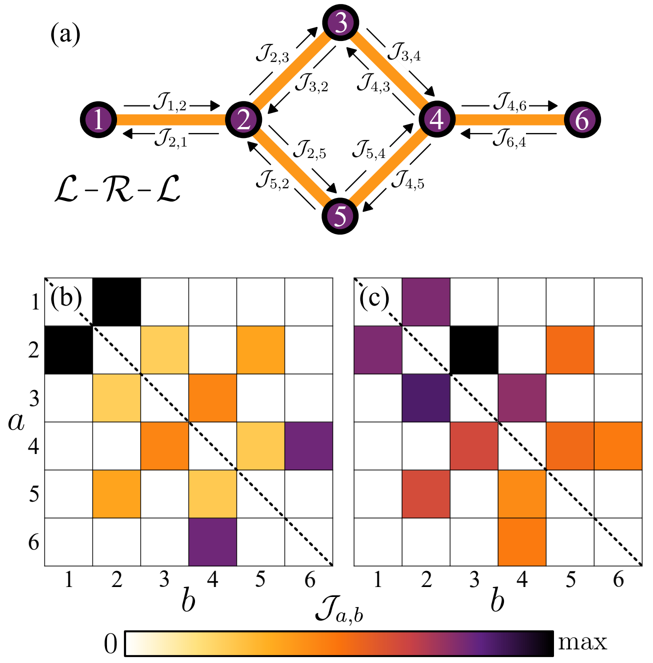


FIG. S3. (a) Graph of the $\mathcal{L}$-$\mathcal{R}$-$\mathcal{L}$ network described in Section ??. The unidirectional electronic flux $\mathcal{J}_{a,b}$ on each edge is marked. Flux matrix $\boldsymbol{\mathcal{J}}$ of the $\mathcal{L}$-$\mathcal{R}$-$\mathcal{L}$ network at steady-state for (b) unithermal and (c) multithermal systems.

To illustrate this observation we construct the steady-state flux matrix $\boldsymbol{\mathcal{J}}$ where $\mathcal{J}_{ab} = \mathcal{J}_{a,b} = k_{a,b}\mathcal{P}_a$ for the ring system with linear attachments drawn in Fig. ??(a). As shown in Fig. ??(b), in the unithermal case, all unidirectional fluxes through a specific connection are equal: $\mathcal{J}_{a,b} = \mathcal{J}_{b,a}$. However, this is not the case for sites that are part of cycles in multithermal systems. While the net flux in the linear attachments vanishes: $\mathcal{J}_{1,2} = \mathcal{J}_{2,1}$ and $\mathcal{J}_{4,6} = \mathcal{J}_{6,4}$, there is an induced current around the inner ring structure ($2 \to 3 \to 4 \to 5 \to 2$) as illustrated by asymmetry in flux matrix in Fig. ??(c). This result gives impetus for further study of thermal control of both directionality and magnitude of of electric currents in complex ET networks.
